# Supplementary material for: Super-resolved imaging based on spatiotemporal wavefront shaping
Source: arXiv:2210.12010 source file (2022-10-21)
Supplement: Supplementary file 1 [file Letter_Vortex_SI_GNoetinger.pdf]

# Super-resolved imaging based on spatiotemporal wavefront shaping
# Supplementary information

Guillaume Noetinger,[1] Samuel Métais,[2] Geoffroy Lerosey,[3] Mathias Fink,[1] Sébastien Popoff,[1] and Fabrice Lemoult[1]

[1]*Institut Langevin, ESPCI Paris, Université PSL, CNRS, 75005 Paris, France*
[2]*Aix Marseille Université, CNRS, Centrale Marseille, Institut Fresnel, Marseille, France*
[3]*Greenerwave, 75002 Paris, France*

## DETAILS OF THE EXPERIMENT

All the experimental protocol and data analysis was carried out using *Python*.

### Set-up

The soundcard I/O device is an *Antelope Orion TB32+* with a total of 32 output channels and 32 input channels. The sampling frequency is 44100 kHz. Thanks to the 'pyaudio' library live emitting/recording is controlled by computer.

*Imaging and excitation lenses.* Inside an anechoic chamber 16 microphones and loudspeakers are disposed in a circle of radius $R = 55$ cm and connected to the soundcard. The distance between each microphone/loudspeaker is thus approximately $\frac{2\pi}{16} \cdot R = 21$ cm. This imposes an upper limit on the wavelength used: to have a satisfiying spatial sampling of a rotating emitter this distance should roughly be of the same order of magnitude than the wavelength.

All the microphones are *t.bone MM-1* pressure recording omnidirectional microphones. They are all connected to their own Microphone Preamp (Antelope MP32) which provides a phantom power supply as well as electronic amplification. All the loudspeakers are 4Ω 3W loudspeakers equipped with one tunable Adafruit PAM8302 class D 2.5W mono amplifier each. The amplifiers are connected to an electrical USB 5V outlet and amplify each outputs of the soundcard, the amplified and impedance matched signal is delivered to the loudspeakers.

In practice the microphone are slightly higher than the loudspeakers of approximately 15cm leading to a small difference of numerical aperture for the illumination (loudpseakers) and collection (microphones) lenses $NA_{ill} \simeq \frac{d}{\sqrt{h_{ls}^2+d^2}} = \frac{0.55}{\sqrt{1.72^2+0.55^2}} = 0.31$ and $NA_{coll} \simeq \frac{d}{\sqrt{h_{mic}^2+d^2}} = \frac{0.55}{\sqrt{1.57^2+0.55^2}} = 0.33$ that we chose to neglect.

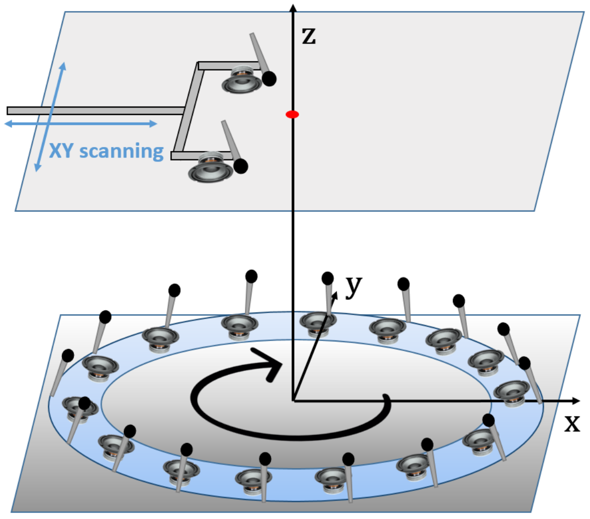


Figure 1. **Sketch of the complete setup:** The ring of loudspeakers and microphones and the two scatterers are depicted. The distance between the two scatterers can be adjusted.

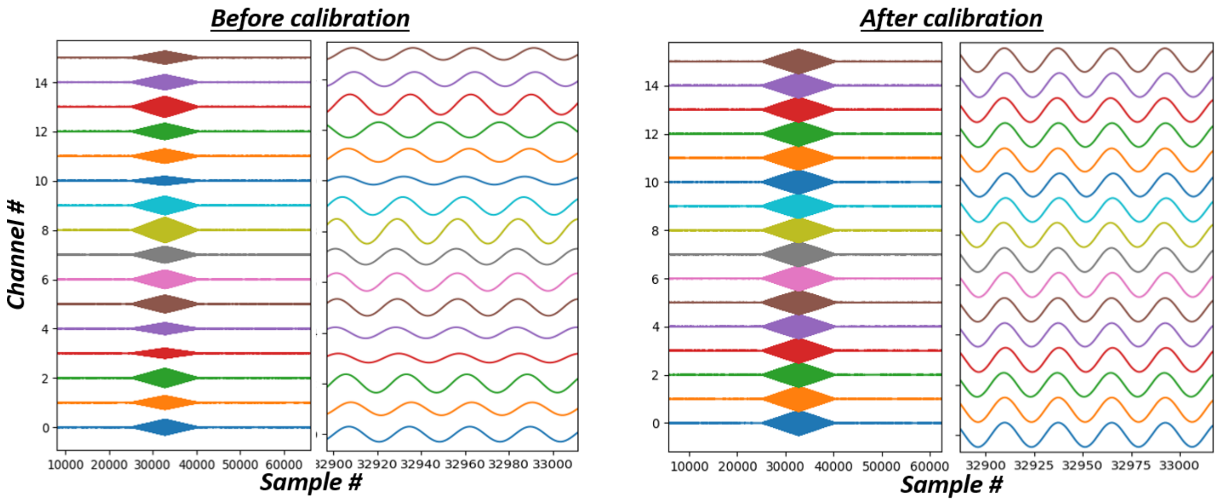


Figure 2. **Calibration procedure - Left:** Signals measured in the focal plane on the rotation axis when each lens's speaker emits a pulse: mismatches in amplitude and phase (as highlighted by temporal zoom) are evidenced. **Right:** After calibration, all signals have same amplitude and phase.

*Active scatterers.* Active scatterers are made with a t.bone MM-1 microphone and a 3W loudspeaker close together at subwavelength scale, here the center of the microphone and loudspeaker are slightly less than 2cm close. Each active scatterer's loudspeaker is connected to the output of a Dynavox HiFi amplifier. We chose not to use another PAM8302 amplifier as for the lense's amplifier to have a better sound quality for the reflection process inexpensively and a simple knob to set the gain. They are fixed at the end of a beam on the translation stage.

*Translation stage* The translation stage is a heavy duty two-axis translation stage with two stepper motors powered with a *Schrittmotor C142* controller interfaced using *pyserial*. Each axis has a total stroke of approximately 1 m which limits the field-of-view of the experiment. This has to be taken under consideration when choosing the wavelength $\lambda$. It should be low enough to allow to have a few $\lambda$ of displacement on each axis.

*Rotating emitter/receiver signal computation.* For each channel corresponding to the rotating emitter a monochromatic signal is multiplied by a gaussian or triangular window centered on the time corresponding to the angular position of the rotating emitter. The width of this window is such that the sum of all time-gated signal corresponds to the desired emission profile of the rotating loudspeaker which is a constant monochromatic signal here. This imposes the width at half-maximum of the windows to be equal to the time between each loudspeaker. The same process is achieved for the receiving channels to mimic a rotating receiver.

## Calibration

All the impedance and gain of the 2.5W amplifiers are slightly different from one another. This induces random, yet deterministic, amplitude and phase differences in the signal sent for each channel. If the same signals were sent simultaneously to every channel there would be no spatial focusing centered on the rotation axis observed. In order to compensate for this effect we performed a calibration step before the experiments.

A microphone on the translation stage (corresponding to one of the active scatterers) is put on the rotation axis. Each lense's loudspeaker sends a pulse (monochromatic signal multiplied by a gaussian window) recorded by the on-axis microphone in the focal plane. The relative height and position of each pulses maximum gives a corrective multiplying factor (gain) and sample shifting (phase) for each channel. Those correcting factor are next applied to the pre-computed signals for each channel. As a consequence, a nice focusing can be observed in the focal plane on the rotation axis if all channels of the lens emit together.

For the experiment with two loudspeakers in the focal plane (used for the active diffusers) the same phenomenon is observed although less pronounced thanks to the higher quality of the amplifier. A similar calibration is performed nevertheless using the same process with the reference microphone being one microphone of the lense.

It is not necessary to perform the same process for the microphones, given the better quality of both the microphones and the pre-amplifier.

## Acquisition process

### *Dynamic configuration*

The emission frequency was chosen considering the compromise between field-of-view and spacing between lens's loudspeakers. It was set to 1600 Hz, this corresponds to a wavelength of 21.4 cm. The rotation frequency was set to 4 Hz with a number of turns set to 4 to allow for averaging.

During the acquisition the scatterers are moved point-by-point with the translation stage on a square grid of 90cm-side with large temporal pauses for mechanical stability. For each point, the sequence of pre-computed signals (namely after calibration) mimicking a rotating source is emitted by the loudspeakers. For the sake of speedness only 4 cycles are emitted. In the meantime, the wavefield in the focal plane is measured by the microphones of the active scatterers. To erase low frequency variations and 50 Hz modulation it is numerically filtered around the emitted frequency with a Butterworth band-pass filter of order 4. The bandwidth of this filter, which has to be large enough to keep the signal with the modulation coming from the rotation, is chosen to be 150 Hz.

The recorded signal is then emitted by the speaker in the focal plane. It is recorded by the lens's microphones and filtered with the same numerical bandpass filter as before. To obtain the signal recorded by a virtually rotating recorder all the signals are multiplied by the temporally shifted gaussian windows.

### *Confocal configuration*

To perform a confocal image with the same setup we should emit a monochromatic signal with all the loudspeaker at the same time with same amplitude and phase (thus requiring the calibration). However, in our case, all the amplifiers cannot send signals at the same time because that would draw too much power from the electrical outlet. We thus apply the superposition theorem to sum up all the signals received in the focal plane when each speaker emits a gaussian pulse. For the receiving part no temporal windowing is applied and all signals are summed together. Finally, only the Fourier transform at the angular frequency $\omega_0$ is kept, thus providing the equivalent of a monochromatic experiment.

### *Experiment with two scatterers in the focal plane*

The code is the same with two scatterers in the focal plane except during the re-emission step. Instead of routing the filtered signal from a single microphone to a single loudspeaker this has to be achieved for another pair of microphone and loudspeaker.

## Building images

To build images at the frequencies $\omega_0 + n\Omega$ with $n \in \mathbb{N}$ from complex data of shape $[N_x, N_y, N_t]$ corresponding to the number of steps in $x$ and $y$ directions and the number of samples (typically $[N_x, N_y, N_t] = [80, 80, 44100]$) the data is first demodulated by multipliying each temporal vector (last dimension) with a monochromatic signal at the carrier frequency $e^{-i\omega_0 t}$.
Then instead of computing the temporal Fourier transform and extracting the value of this transform at $n\Omega$ we compute the Fourier coefficients for the appropriate $n$. To do this we multiply each temporal vector (last dimension) with a monochromatic signal $e^{-in\Omega t}$, sum along this dimension and normalize by $N_t$.

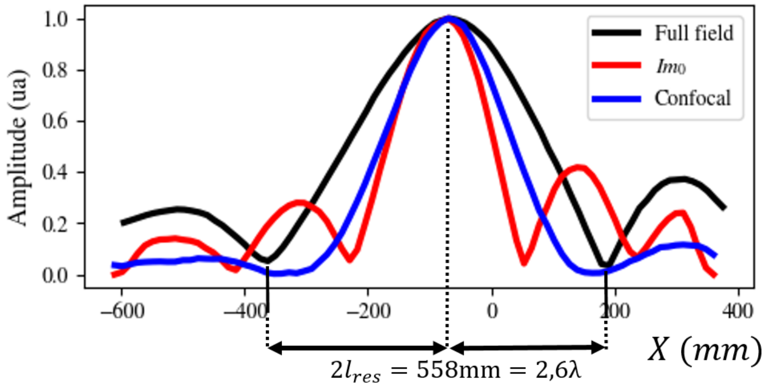


Figure 3. **Experimental amplitude profiles** (in absolute value) of the full-field $PSF$, the confocal $PSF$ and $PSF_0$ the point-spread function at $\omega_0$ in the dynamic case. The zeroes of $PSF_0$ seem approximately two times closer to the origin compared to the two other scenarii.

## RESULTS

### Full field resolution

The diffraction limited focal spot of a full-field microscope with a regular microscope objective (*ie.* a full lens) is given by the Fourier transform of the pupil function [1] :

$$PSF(r) \propto \int_0^1 J_0\left(\frac{2\pi NA}{\lambda} rr'\right) r'dr' \propto \frac{J_1\left(\frac{2\pi NA}{\lambda} r\right)}{\frac{2\pi NA}{\lambda} r} \tag{1}$$

where $r'$ is the normalized integration variable corresponding to the annular/radial contribution of the pupil to the focal spot. The first zero of this function corresponds to $\frac{2\pi NA}{\lambda} r = 3.8$. According to Rayleigh criterion the resolution limit is then $l_{\text{res}} = 1.22 \frac{\lambda}{2\,NA}$
In our case the pupil function is a thin ring and thus the $PSF$ reduces to a single element of the previous integral:

$$PSF(r) \propto J_0\left(\frac{2\pi NAr}{\lambda}\right) \tag{2}$$

The first zero of this function corresponds to $\frac{2\pi NA}{\lambda} r = 2.4$ [2] so $l_{\text{res}} = 0.76 \frac{\lambda}{2\,NA}$ this is equal to 27.1 cm here. The fact that the imaging resolution is given by this criterion comes from reciprocity [3].

Experimentally, this monochromatic configuration corresponds to the wave field measured in the focal plane at the harmonic $n = 0$. A radial profile of the absolute value of the latter is represented in Fig. 3. The difference of position of the two first zeros corresponding to $2l_{\text{res}}$ is measured t (see Figure 3) and gives $l_{\text{res}} = 27.9 \simeq 28$cm which corresponds to the previous calculation.

### Confocal resolution

When performing a confocal scenario, the wave-field is focused during the emission and the reception step. As a consequence the round trip implies a squaring of the full-field $PSF$. Experimentally, the confocal image is obtained after a full-scan of the focal plane by the scatterer. Again, a radial profile of the absolute value of the confocal $PSF$ is shown in Figure 3. The zeroes of the confocal experiment are almost at the same positions as in the full-field, they might be a little closer to the center of the spot, this could be explained by the slightly higher numerical aperture of the imaging lense (see ) . So according to the Rayleigh criterion the resolution of confocal is not enhanced compared to the full-field scenario. Nevertheless, due to the squaring of the full-field $PSF$, the focal spot presents lower side-lobes and a thinner spot when considering a full-width at half maximum as the new criterion.

By acquiring various confocal images with two scatterers separated by distances from 30 cm down to 10 cm, we can quantify the resolution of our confocal setup. At 22.5 cm, the two diffusers are almost indistinguishable (see Figure 4) so we estimated the resolution limit in this particular imaging configuration at 22cm.

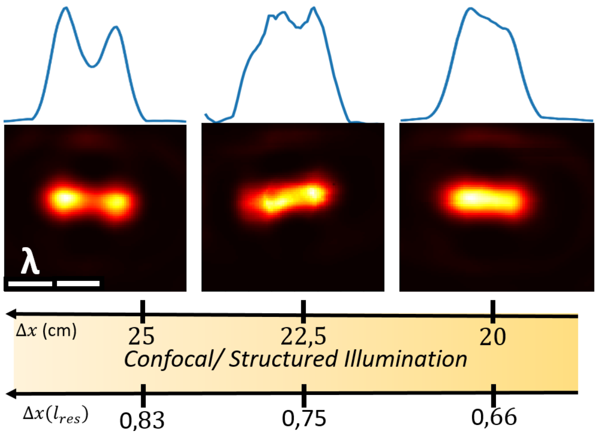


Figure 4. **Confocal images of two diffusers with various separation distance** The field of view is $90 \times 90$cm

**Observation of the resolution enhancement in the dynamic case**

In the dynamic confocal scenario, each point of the focal plane is associated to a transient wavefield. A noteworthy observation can be made from the snapshot of such transient wavefield. Indeed, as shown in Figure 5 the apparent wave-scale in the backscattered signals since twice smaller compared to the focal plane.

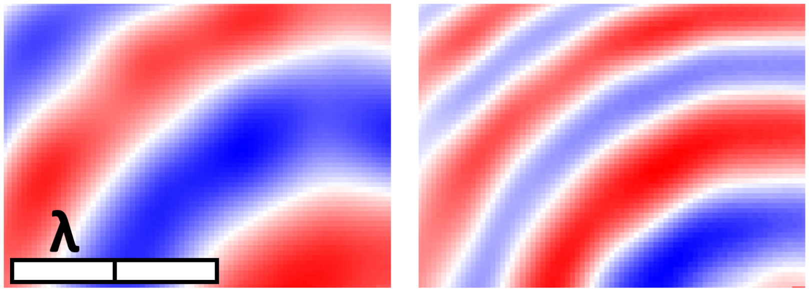


Figure 5. **Images of the temporal fields** with a single diffuser in the focal plane (left) and backscattered (right) corresponding to the $PSF$ acquisition. It is extracted from a full movie where the rotation of the emission center (here at the bottom right of each image) can be observed.

This observation in the time domain is actually equivalent to the observations made in the main text when comparing the fields at different harmonic in figure 2 of the main text. As an illustration, a radial profile of the $PSF_0$ corresponding to the backscattered field at harmonic $n = 0$ is shown in figure 4. The zeros have moved closer to the center as expected by the apparent shorter wavelength. However the side-lobes level have come back to the same level as in the full-field scenario and is therefore higher than the confocal one.

Let us switch to a Fourier standpoint and consider the spatial frequencies transmitted by the system. The image $Im_0$ is built compared to the confocal one by keeping only the combination of illumination and collection wavevectors with highest $NA$. Each of them is limited by the diffraction to a longitudinal contribution of $1.22\frac{\lambda}{2\,NA}$ (See Figure 6a). This is exactly the same as in diffuse tomography [4] and leads to an enhancement in resolution by a factor of two. The same explanation has been proposed for structured illumination [5].

In the dynamic configuration not all of the pupil's recorder are working at the same time. As a consequence with our 'dynamic filter' we extract only the high spatial frequencies components of the confocal image in the dynamic image $Im_0$. In the case of the confocal image the high spatial frequencies channel are fewer than the low frequencies channel which is not favorable to inversion.

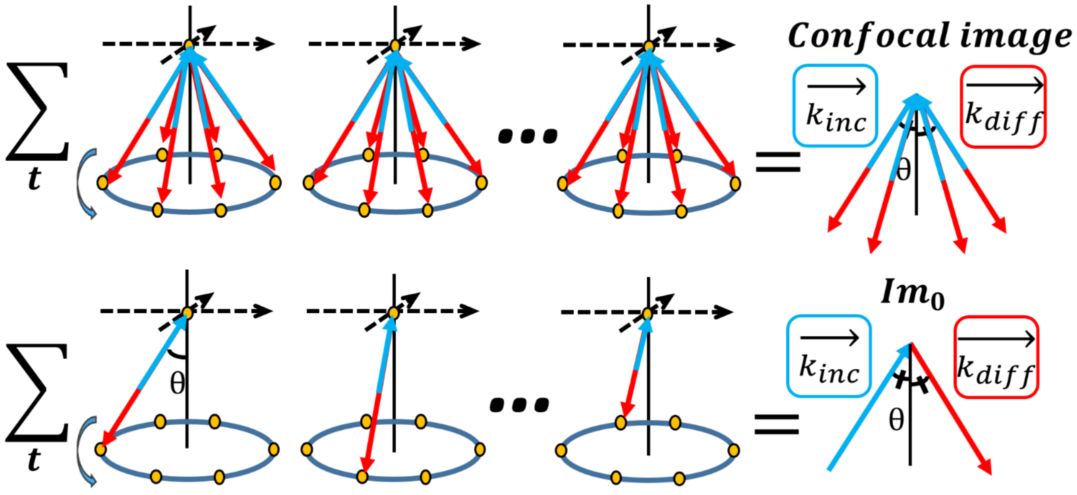


Figure 6. **Explanations of the resolution enhancement** with an annular acoustic lense made of 6 lenses and microphones **(a) Construction of the confocal (top) and $Im_0$ (bottom) images with dynamic signals** Using the temporal Fourier transform and keeping the image at the carrier frequency is equivalent to calculating the temporal sum of the signals to a proportionality factor

## NUMERICAL ANALYSIS

All the numerical analysis was carried out using *Matlab*.

### Details of the numerical calculations

To write the field in the focal plane, we need to introduce the temporal Green's function $G_0(\mathbf{r}, t|\mathbf{r_s}, t_0)$ relating a source at position $\mathbf{r_s}$ emitting a Dirac at time $t_0$ and an observer at position $\mathbf{r}$ in the focal plane. For scalar waves in 3D it corresponds to a spherical wavefunction which mathematically writes:

$$G_0(\mathbf{r}, t|\mathbf{r_s}, t_0) = \frac{\delta\left(t - t_0 - \frac{||\mathbf{r}-\mathbf{r_s}||}{c}\right)}{4\pi||\mathbf{r} - \mathbf{r_s}||} \tag{3}$$

By applying the superposition theorem and knowing the signal emitted by each speaker it is straightforward to numerically obtain the signal received on each point of the focal plane since the propagation amounts to a convolution with the temporal Green's function. For the sake of time efficiency the calculations are actually performed in the Fourier domain where the convolution is a simple multiplication. We come back to the time domain at the end by applying an inverse Fourier transform.

For the back-scattered step, the same procedure as in the experiment is applied. Each signal obtained in the focal plane is back-propagated by the use of the same free space Green's function toward the position of the receivers. Then, the signals are time gated in order to emulate the rotation of a receiver as in the experiment. For each position in the focal plane, we ends up with a single temporal signal.

Each of these transient signals exhibits the same temporal modulation as any signal considered in the article. Its Fourier spectrum is non-zero only on the discrete set of frequencies $\omega_0 + n\Omega$, as shown in the spectrum of figure 1(b) in the main text. As a consequence, it is sufficient to solely represent the data corresponding to this discrete set of frequencies.

### Comparison with the simulation and experiment

We witness a good *qualitative* agreement between the numerical analysis and the experiment both in the focal plane and the backscattered field (See Figure 7). The phases of the vortices only differ by a constant phase factor and a

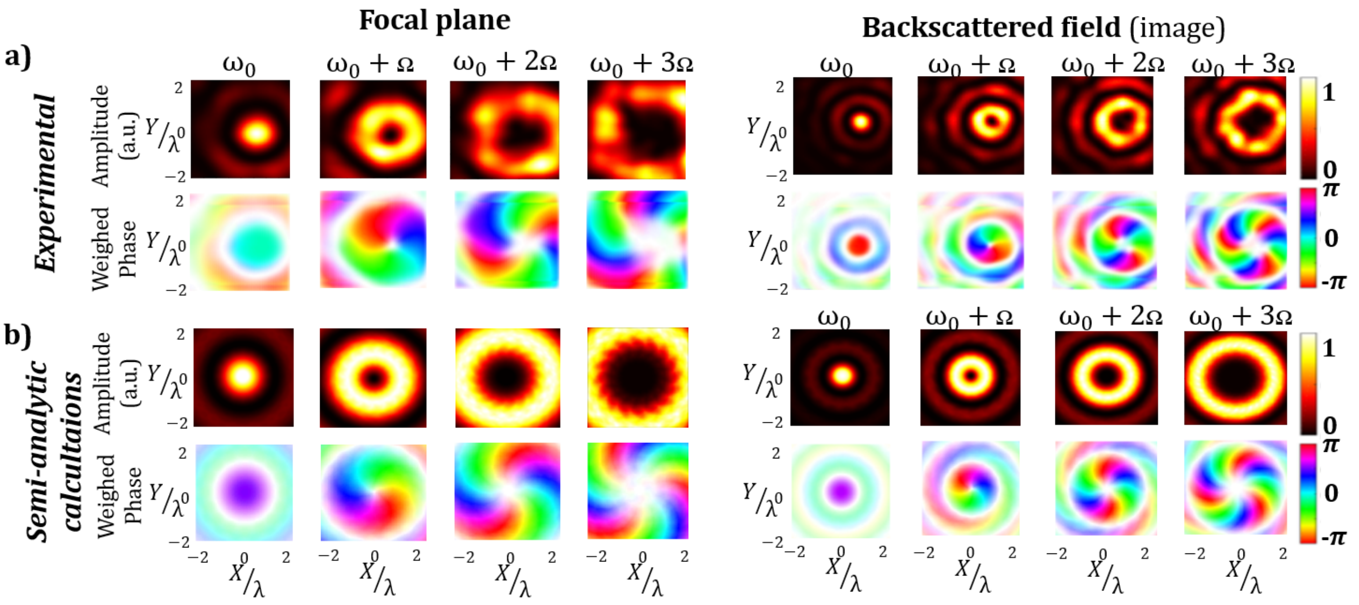


Figure 7. Comparison of the experimental data and the simulated field **(a)** : Experimental data : amplitude and weighted phase spatial representation of the field in the focal plane and the backscattered field for the first four harmonic signals **(b)** : Semi-analytic calculations data : amplitude and weighted phase spatial representation of the field in the focal plane and the backscattered field for the first four harmonic signals

constant shift. There is a slight difference in the width of the vortex rings due to some minor parameter's differences in the experimental and numerical parameters that were not optimized for a perfect quantitative agreement.

## RECONSTRUCTION

### Detailed procedure

The image of a single scatterer at harmonic angular frequency $\omega_0 + n\Omega$ is saved and used as the $PSF_n$ of the system. Its inverse $iPSF_n$ is then computed in the spatial Fourier domain using Tikhonov regularization. Typically the following formula is applied:

$$\widehat{iPSF}_n(\mathbf{k}) = \left(\widehat{PSF}_n^*(\mathbf{k}) \cdot \widehat{PSF}_n(\mathbf{k}) + \sigma\right)^{-1} \cdot \widehat{PSF}_n^*(\mathbf{k})$$

Even with the apodization and regularization the level of high frequencies artifacts would be too high for each image so a multipliying cutoff filter is added. A circularly symmetric gate window is chosen. It cuts all the spatial frequencies above $(1+f_{super}) \cdot \frac{4 \cdot NA}{\lambda}$ where $f_{super}$ is a tunable factor corresponding to the maximum possible bandwidth extension which means superresolution.

Each image of the two scatterers are also spatially Fourier transformed and multiplied by $\widehat{iPSF}_n(\mathbf{k})$. Eventually, an inverse spatial Fourier transform allows retrieving a reconstructed image in the real space $Obj_n(\mathbf{r})$.

### Choice of the reconstruction parameters

Various values for $\sigma$ and $f_{super}$ have been tried. Picking the right value is always arbitrary like the definition of resolution criterions. To make a choice we consider a compromise between the ability to distinguish two points and the introduction of reconstruction artifacts . First the superresolution factor was arbitrarily set to a value of 50% which means a cut-off for spatial frequencies above $\frac{6 \cdot NA}{\lambda}$ equivalent to a lateral resolution of 9.7 cm which would allow to reconstruct all the images with two scatterers.

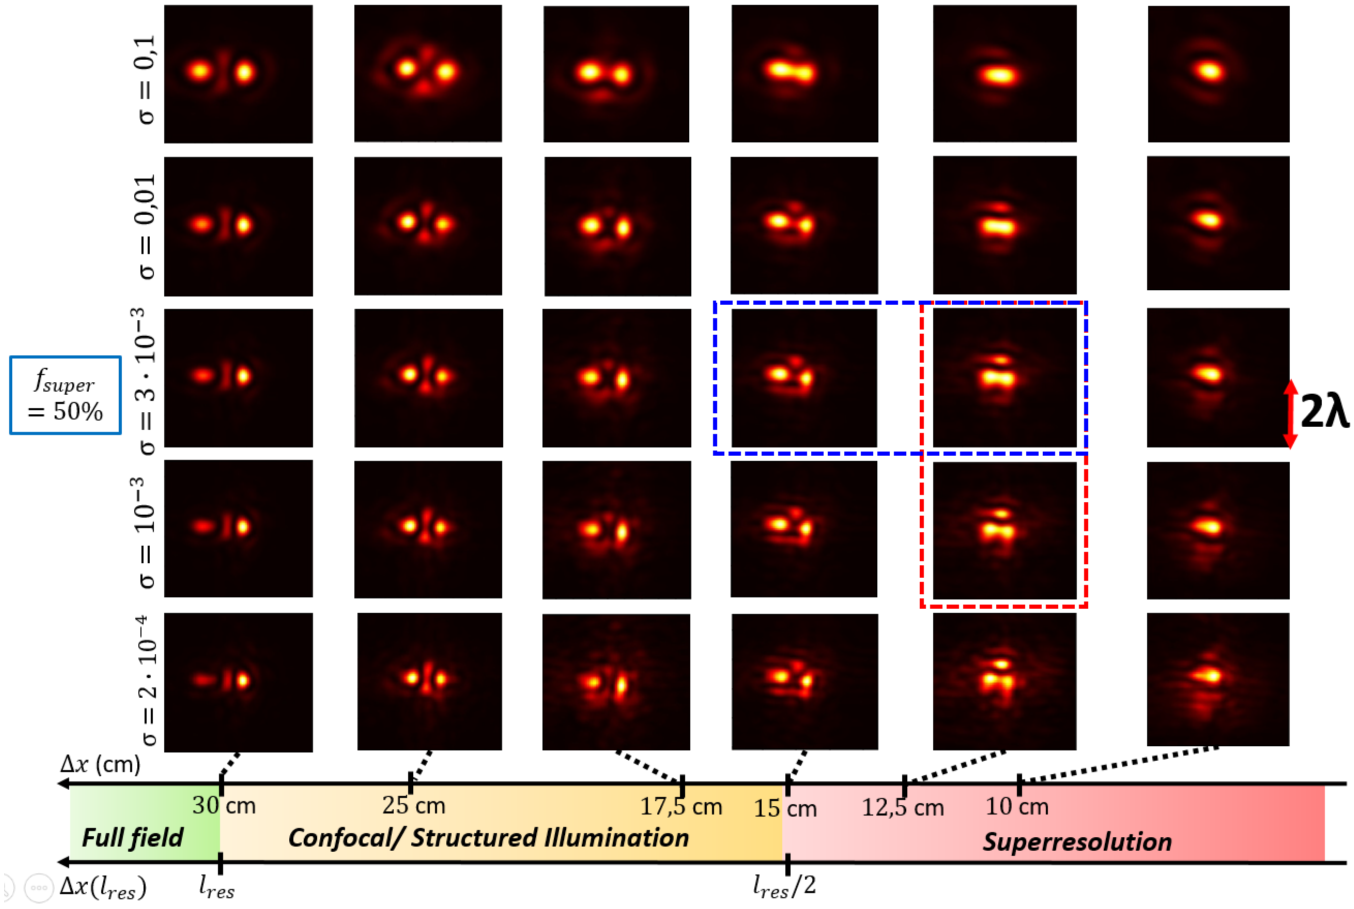


Figure 8. Reconstructed images for various parameters $\sigma$
On the first row the SNR is chosen to be low, we see that this does not allow for a good reconstruction. For the middle row ($\sigma = 3 \cdot 10^{-3}$) the two diffusers can be really separated for 15cm and distinguished for 12.5cm with reconstruction artifacts (blue box), if $\sigma$ decreases again the level of artifacts becomes too high (red box).

The inversion is then performed for different values of $\sigma$ chosen on a logarithmic scale from 0.1 which is equivalent to a low signal to noise ratio of 10 to $1 \cdot 10^{-4}$. In figure 8 many reconstructed images are shown for various values of sigma.

The final choice ended up to be a SNR of $3 \cdot 10^{-3}$. This value allows to distinguish two scatterers at a 15cm-distance using the Rayleigh criterion without a high level of artifacts. It also allows to distinguish scatterers at a distance of 12.5 cm using *Sparrow* criterion with the presence of a small reconstruction artifact above the two scatterers. We chose not to consider a smaller value for $\sigma$ since it does not allow a significant improvement in resolution and increases the level of artifacts for this last experiments.

After this choice, attempts without success have been made to increase $f_{super}$ in order to obtain a higher lateral resolution so the final value staid at 50%.

[1] M. Born and E. Wolf, *Principles of Optics*, 7th ed. (Cambridge University Press, 1999).
[2] M. Abramowitz and I. Stegun, *Handbook of Mathematical functions*, 1st ed. (National Bureau of Standards, 1964).
[3] C. J. R. Sheppard and T. Wilson, Reciprocity and equivalence in scanning microscopes, J. Opt. Soc. Am. A **3**, 755 (1986).
[4] O.Haeberlé, K.Belkebir, H.Giovaninni, and A.Sentenac, Tomographic diffractive microscopy: basics, techniques and perspectives, Journal of Modern Optics **57**, 686 (2010).
[5] M. G. L. Gustafsson, Surpassing the lateral resolution limit by a factor of two using structured illumination microscopy, Journal of Microscopy **198**, 82 (2001).
